# Supplementary material for: Minimax Demographic Group Fairness in Federated Learning
Source: arXiv:2201.08304 source file (2022-01-25)
Supplement: Supplementary file 1 [file appendix.tex]

\appendix

\section{Appendix: Proofs}\label{proofs_sup}

\input{appendix/lemma_objectives}
\input{appendix/lemma_convergence}

\section{Appendix: Experiments}\label{more_results}
\input{appendix/more_results}
